# Supplementary material for: UDAPose: Unsupervised Domain Adaptation for Low-Light Human Pose Estimation
Source: arXiv:2604.10485 source file (2026-04-12)
Supplement: Supplementary file 6 [file lambda.tex]

\input{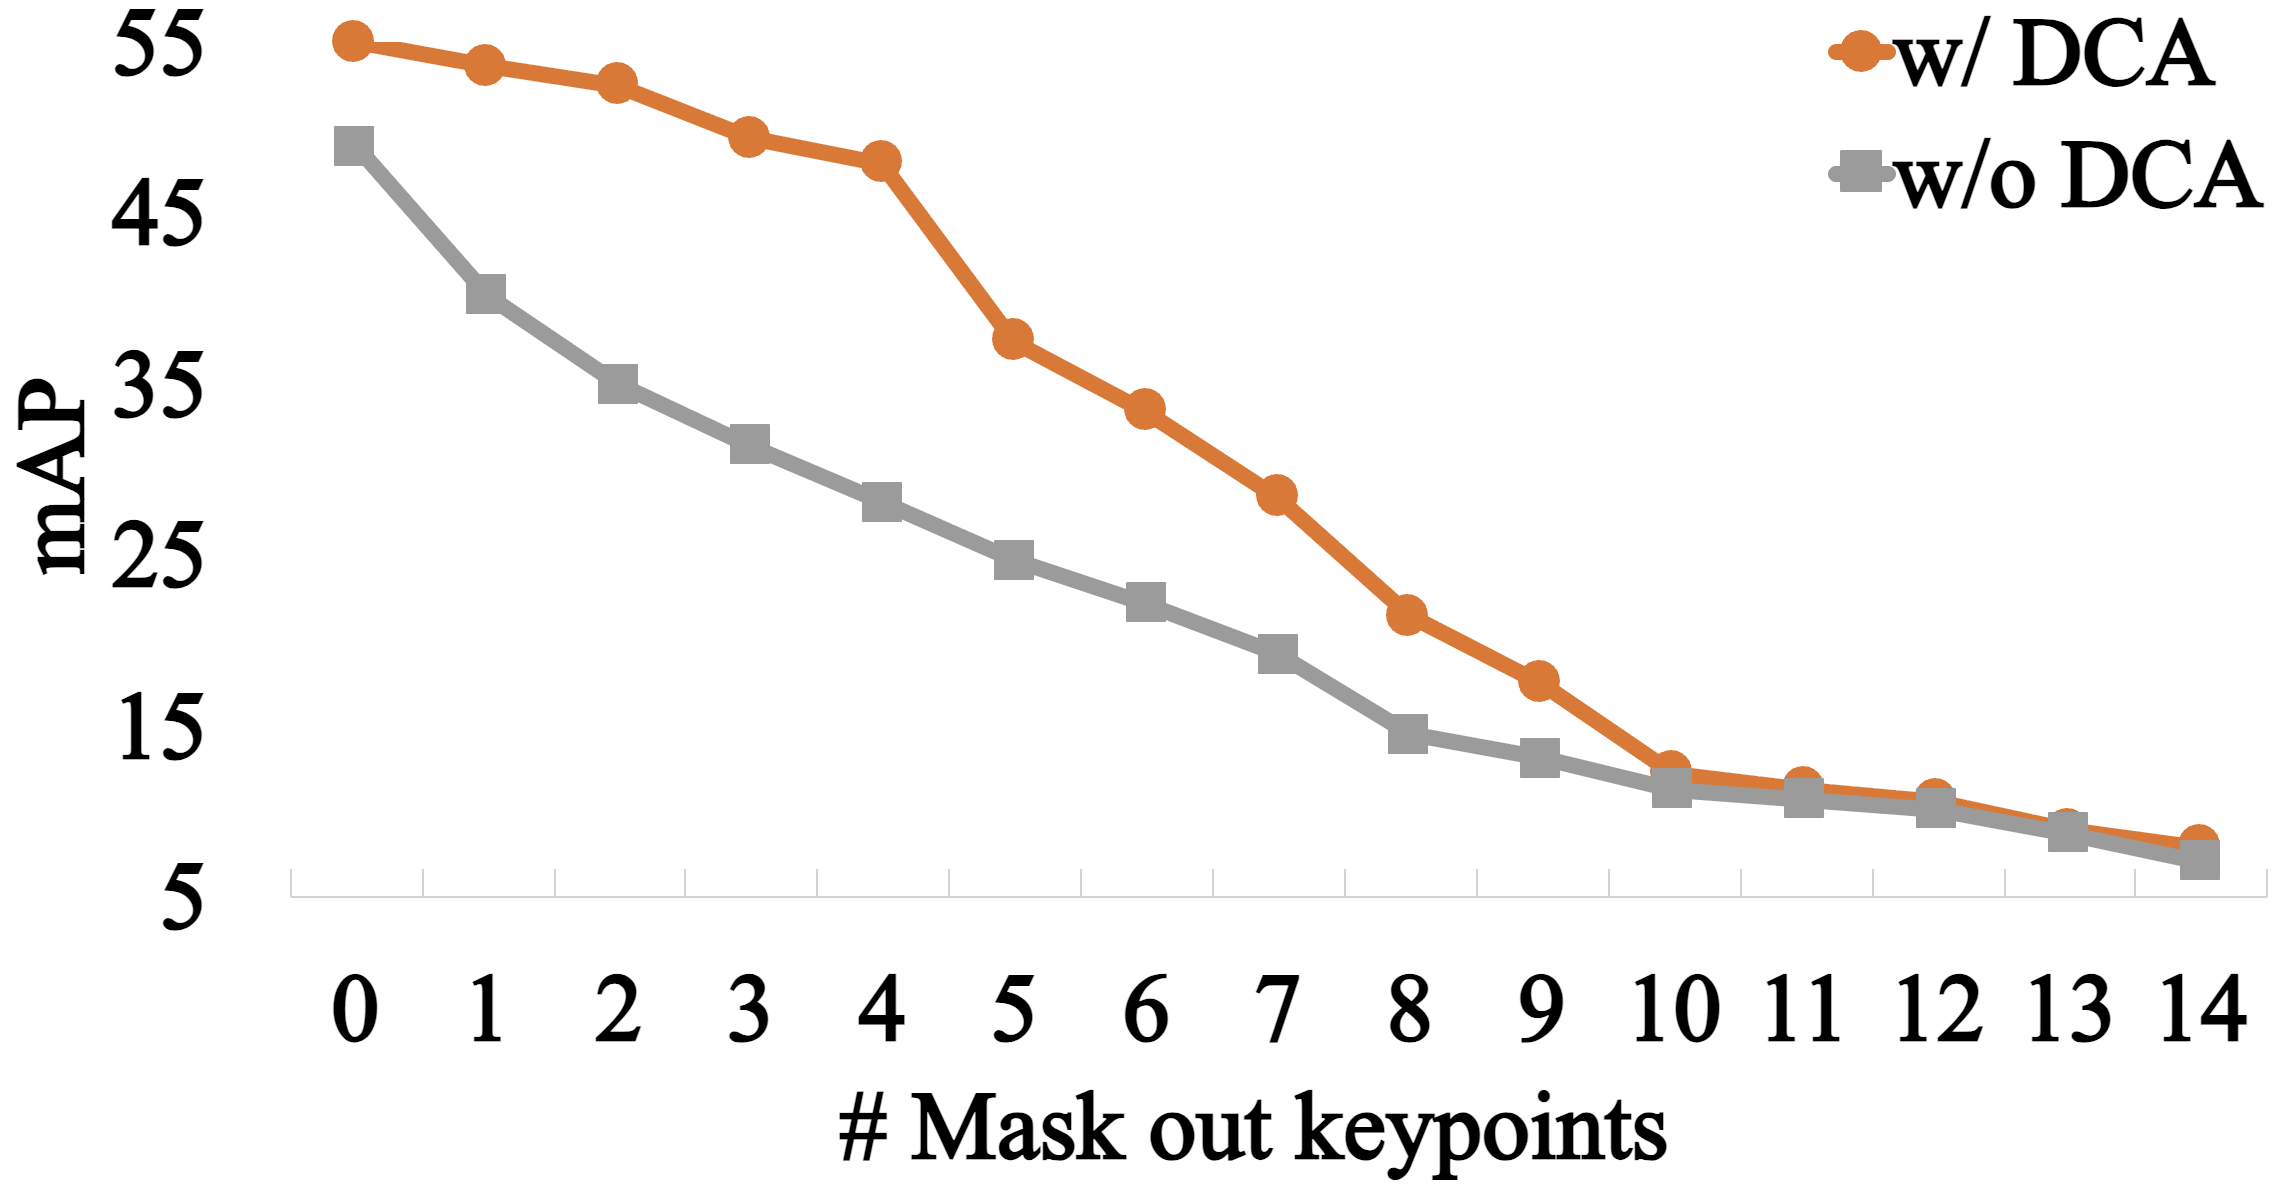}

\section{Evaluation of $\lambda$ and DCA}
\haopeng{NEW ADDED section}
As in~\cref{fig:lambda}, larger $\lambda$ emphasizes high-frequency details but may fail to keep content consistency (lower SSIM), while smaller $\lambda$ weakens low-light realism and reduces mAP. We choose $\lambda = 4 \times 10^{-4}$.

We conduct a masking evaluation on ExLPose-OCN (A7M3) by progressively masking random keypoints. DCA consistently outperforms the baseline (no DCA) when a small number of keypoints are missing, while the gap narrows where most keypoints are masked as shown in~\cref{fig:mask}.
